# Supplementary material for: Predicting fuel research octane number using Fourier-transform infrared absorption spectra of neat hydrocarbons
Source: arXiv:1606.07122 source file (2016-06-22)
Supplement: Supplementary file 1 [file Supplemental_Material.pdf]

## Supplemental Material

### 1. Lists of fuel mixtures

This study considered a total of 134 fuel blends consisting of various mixtures *n*-heptane, isooctane, methylcyclohexane, toluene, 1-hexene, and ethanol taken from the literature [1–4]. Tables 1–5 provide the makeup of these mixtures in terms of volume fraction, as well as the RONs measured experimentally by the sources.

| ID | *n*-heptane (vol. %) | isooctane (vol. %) | MCH (vol. %) | toluene (vol. %) | 1-hexene (vol. %) | RON |
|---|---|---|---|---|---|---|
| 2 | 60 | 10 | 10 | 10 | 10 | 41.0 |
| 3 | 50 | 50 | | | | 48.3 |
| 4 | 50 | | 50 | | | 43.8 |
| 5 | 50 | | | 50 | | 64.1 |
| 6 | 50 | | | | 50 | 40.3 |
| 7 | 20 | 20 | 20 | 20 | 20 | 75.0 |
| 8 | 10 | 60 | 10 | 10 | 10 | 87.1 |
| 10 | 10 | 10 | 60 | 10 | 10 | 74.4 |
| 11 | | 50 | 50 | | | 86.4 |
| 13 | 10 | 10 | 10 | 60 | 10 | 95.7 |
| 14 | | 50 | | 50 | | 110.5 |
| 15 | | | 50 | 50 | | 91.5 |
| 16 | 10 | 10 | 10 | 10 | 60 | 75.8 |
| 18 | | 50 | | | 50 | 88.2 |
| 19 | | | 50 | | 50 | 74.2 |
| 20 | | | | 50 | 50 | 92.5 |

Table 1: Blends of *n*-heptane, isooctane, methylcyclohexane (MCH), toluene, and 1-hexene considered in this work taken from Perez et al. [1].

| ID | $n$-heptane (vol. %) | isooctane (vol. %) | toluene (vol. %) | ethanol (vol. %) | RON |
|---|---|---|---|---|---|
| PRF20 | 80 | 20 | | | 20 |
| PRF40 | 60 | 40 | | | 40 |
| PRF55 | 45 | 55 | | | 55 |
| PRF85 | 15 | 85 | | | 85 |
| H20T10 | 20 | 70 | 10 | | 82.8 |
| H20T20 | 20 | 60 | 20 | | 84.9 |
| H20T40 | 20 | 40 | 40 | | 89.8 |
| H20T60 | 20 | 20 | 60 | | 93.9 |
| PRF80 | 80 | 20 | | | 80 |
| H20E1 | 20 | 79 | | 1 | 80.5 |
| H20E5 | 20 | 75 | | 5 | 84.4 |
| H20E10 | 20 | 70 | | 10 | 87.9 |
| H20E20 | 20 | 60 | | 20 | 94.1 |
| PRF70 | 70 | 30 | | | 70 |
| H30E1 | 30 | 69 | | 1 | 70.6 |
| H30E5 | 30 | 65 | | 5 | 73.2 |
| H30E10 | 30 | 60 | | 10 | 78.7 |
| H60E20 | 30 | 50 | | 20 | 85.1 |
| H60E40 | 60 | | | 40 | 71.4 |
| H55E45 | 55 | | | 45 | 78 |
| H50E50 | 50 | | | 50 | 84.7 |
| H45E55 | 45 | | | 55 | 89.7 |
| H40E60 | 40 | | | 60 | 94.4 |
| T1 | 40 | 45 | 10 | 5 | 67.1 |
| T2 | 20 | 50 | 10 | 20 | 94.7 |
| T3 | 20 | 30 | 30 | 20 | 97 |
| T4 | 40 | 10 | 30 | 20 | 80.8 |
| T5 | 30 | 45 | 20 | 5 | 79.6 |
| T6 | 30 | 27.5 | 30 | 12.5 | 85.3 |
| T7 | 30 | 37.5 | 20 | 12.5 | 83.8 |
| T8 | 40 | 25 | 30 | 5 | 71.8 |
| T9 | 30 | 47.5 | 10 | 12.5 | 81.6 |
| T10 | 20 | 45 | 30 | 5 | 90.2 |
| T11 | 30 | 37.5 | 20 | 12.5 | 83.8 |
| T12 | 40 | 30 | 10 | 20 | 78.3 |
| T13 | 20 | 65 | 10 | 5 | 86.1 |
| T14 | 40 | 27.5 | 20 | 12.5 | 74.8 |
| T15 | 20 | 47.5 | 20 | 12.5 | 92.3 |
| T16 | 30 | 30 | 20 | 20 | 87.9 |
| T17 | 30 | 37.5 | 20 | 12.5 | 83.8 |

Table 2: Blends of $n$-heptane/isooctane (PRFs), $n$-heptane/isooctane/toluene, $n$-heptane/isooctane/ethanol, $n$-heptane/ethanol, and $n$-heptane/isooctane/toluene/ethanol considered in this work taken from Truedsson et al. [3, 4].

| ID | $n$-heptane (vol. %) | isooctane (vol. %) | toluene (vol. %) | ethanol (vol. %) | RON |
|---|---|---|---|---|---|
| TE10 | | | 90 | 10 | 112.8 |
| TE20 | | | 80 | 20 | 110.9 |
| TE40 | | | 60 | 40 | 108.6 |
| TE60 | | | 40 | 60 | 108.1 |
| TE80 | | | 20 | 80 | 107.9 |
| TRF91-15 | 12.4 | 72.6 | 15 | | 91.0 |
| TRF91-30 | 17 | 53.2 | 29.8 | | 91.3 |
| TRF91-45 | 20.3 | 34.7 | 45 | | 91.1 |

Table 3: Blends of toluene/ethanol and $n$-heptane/isooctane/toluene (TRF) considered in this work taken from Foong et al. [2].

| ID | $n$-heptane (vol. %) | isooctane (vol. %) | ethanol (vol. %) | RON |
|---|---|---|---|---|
| PRF0-E30 | 70 | | 30 | 54.3 |
| PRF0-E40 | 60 | | 40 | 69.7 |
| PRF0-E50 | 50 | | 50 | 83.8 |
| PRF0-E60 | 40 | | 60 | 94.7 |
| PRF0-E70 | 30 | | 70 | 101.6 |
| PRF0-E80 | 20 | | 80 | 104.7 |
| PRF0-E90 | 10 | | 90 | 106.5 |
| PRF10-E20 | 72 | 8 | 20 | 45.9 |
| PRF10-E30 | 63 | 7 | 30 | 61.1 |
| PRF10-E40 | 54 | 6 | 40 | 75.6 |
| PRF10-E50 | 45 | 5 | 50 | 87.6 |
| PRF10-E60 | 36 | 4 | 60 | 96.6 |
| PRF20-E20 | 64 | 16 | 20 | 53.3 |
| PRF20-E30 | 56 | 14 | 30 | 67.4 |
| PRF20-E40 | 48 | 12 | 40 | 80.7 |
| PRF20-E50 | 40 | 10 | 50 | 91.5 |
| PRF20-E60 | 32 | 8 | 60 | 99.1 |
| PRF20-E80 | 16 | 4 | 80 | 105.8 |
| PRF30-E10 | 63 | 27 | 10 | 46.5 |
| PRF30-E20 | 56 | 24 | 20 | 60.8 |
| PRF30-E30 | 49 | 21 | 30 | 74.2 |
| PRF30-E40 | 42 | 18 | 40 | 85.5 |
| PRF30-E50 | 35 | 15 | 50 | 94.7 |
| PRF40-E10 | 54 | 36 | 10 | 55 |
| PRF40-E20 | 48 | 32 | 20 | 68.5 |
| PRF40-E30 | 42 | 28 | 30 | 80.6 |
| PRF40-E40 | 36 | 24 | 40 | 90.4 |
| PRF40-E50 | 30 | 20 | 50 | 97.9 |
| PRF40-E60 | 24 | 16 | 60 | 102.7 |
| PRF40-E80 | 12 | 8 | 80 | 106.6 |
| PRF50-E10 | 45 | 45 | 10 | 63.8 |
| PRF50-E20 | 40 | 40 | 20 | 75.8 |
| PRF50-E30 | 35 | 35 | 30 | 86.4 |
| PRF50-E40 | 30 | 30 | 40 | 94.5 |
| PRF60-E10 | 36 | 54 | 10 | 72.6 |
| PRF60-E20 | 32 | 48 | 20 | 83.5 |
| PRF60-E30 | 28 | 42 | 30 | 92 |
| PRF60-E40 | 24 | 36 | 40 | 98.9 |
| PRF60-E60 | 16 | 24 | 60 | 105.5 |
| PRF60-E80 | 8 | 12 | 80 | 107.6 |
| PRF70-E10 | 27 | 63 | 10 | 80.9 |

| | | | | |
|---|---|---|---|---|
| PRF70-E20 | 24 | 56 | 20 | 90.3 |
| PRF70-E30 | 21 | 49 | 30 | 97.4 |
| PRF80-E10 | 18 | 72 | 10 | 89.5 |
| PRF80-E20 | 16 | 64 | 20 | 97 |
| PRF80-E40 | 12 | 48 | 40 | 105.7 |
| PRF80-E60 | 8 | 32 | 60 | 107.7 |
| PRF80-E80 | 4 | 16 | 80 | 108.3 |
| PRF90-E5 | 9.5 | 85.5 | 5 | 94.1 |
| PRF90-E10 | 9 | 81 | 10 | 97.6 |
| PRF90-E20 | 8 | 72 | 20 | 103.6 |
| PRF100-E10 | | 90 | 10 | 106.8 |
| PRF100-E20 | | 80 | 20 | 109.4 |
| PRF100-E40 | | 60 | 40 | 110.2 |
| PRF100-E60 | | 40 | 60 | 109.6 |
| PRF100-E80 | | 20 | 80 | 109 |

Table 4: Blends of $n$-heptane, isooctane, and ethanol considered in this work taken from Foong et al. [2].

| ID | $n$-heptane (vol. %) | isooctane (vol. %) | toluene (vol. %) | ethanol (vol. %) | RON |
|---|---|---|---|---|---|
| TRF91-15-E10 | 11.16 | 65.34 | 13.5 | 10 | 97.8 |
| TRF91-15-E20 | 9.92 | 58.08 | 12 | 20 | 102.6 |
| TRF91-15-E40 | 7.44 | 43.56 | 9 | 40 | 107.1 |
| TRF91-15-E60 | 4.96 | 29.04 | 6 | 60 | 107.7 |
| TRF91-15-E80 | 2.48 | 14.52 | 3 | 80 | 107.8 |
| TRF91-30-E10 | 15.3 | 47.88 | 26.82 | 10 | 97 |
| TRF91-30-E20 | 13.6 | 42.56 | 23.84 | 20 | 101.4 |
| TRF91-30-E40 | 10.2 | 31.92 | 17.88 | 40 | 106 |
| TRF91-30-E60 | 6.8 | 21.28 | 11.92 | 60 | 107.1 |
| TRF91-30-E80 | 3.4 | 10.64 | 5.96 | 80 | 107.5 |
| TRF91-45-E10 | 18.27 | 31.23 | 40.5 | 10 | 96 |
| TRF91-45-E20 | 16.24 | 27.76 | 36 | 20 | 100.2 |
| TRF91-45-E40 | 12.18 | 20.82 | 27 | 40 | 104.6 |
| TRF91-45-E60 | 8.12 | 13.88 | 18 | 60 | 106.3 |
| TRF91-45-E80 | 4.06 | 6.94 | 9 | 80 | 107.1 |

Table 5: Blends of $n$-heptane, isooctane, toluene, and ethanol considered in this work taken from Foong et al. [2].

## References

[1] P. L. Perez, A. L. Boehman, Experimental investigation of the autoignition behavior of surrogate gasoline fuels in a constant-volume combustion bomb apparatus and its relevance to HCCI combustion, Energy Fuels 26 (10) (2012) 6106–6117. doi:10.1021/ef300503b.

[2] T. M. Foong, K. J. Morganti, M. J. Brear, G. da Silva, Y. Yang, F. L. Dryer, The octane numbers of ethanol blended with gasoline and its surrogates, Fuel 115 (2014) 727–739. doi:10.1016/j.fuel.2013.07.105.

[3] I. Truedsson, The HCCI Fuel Number: Measuring and Describing Auto-ignition for HCCI Combustion Engines, Ph.D. thesis, Lund University (Apr. 2014).

[4] I. Truedsson, W. Cannella, B. Johansson, M. Tuner, Development of new test method for evaluating HCCI fuel performance, SAE Technical Paper 2014-01-2667 (Oct. 2014). doi:10.4271/2014-01-2667.
